# Supplementary material for: Evidence for (and Against) Progenitor Bias in the Size Growth of Compact Red Galaxies
Source: arXiv:1411.6736 source file (2014-11-26)

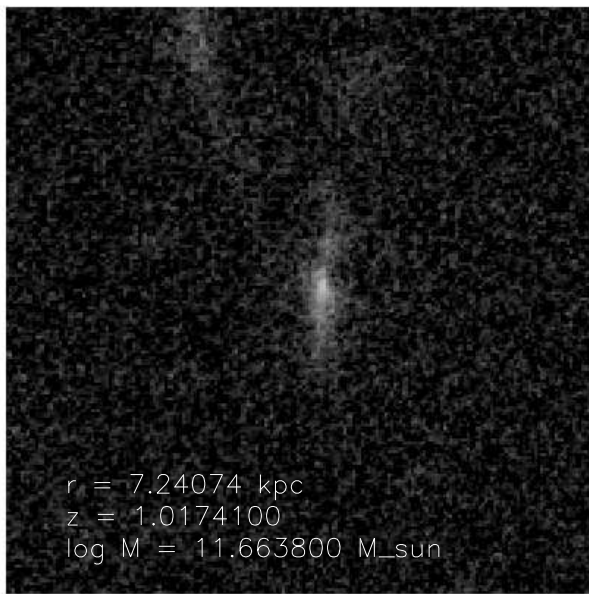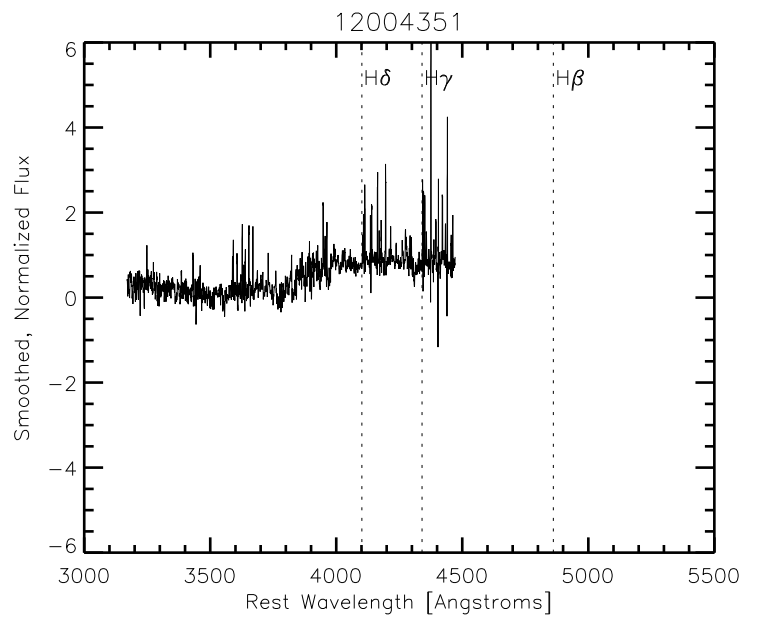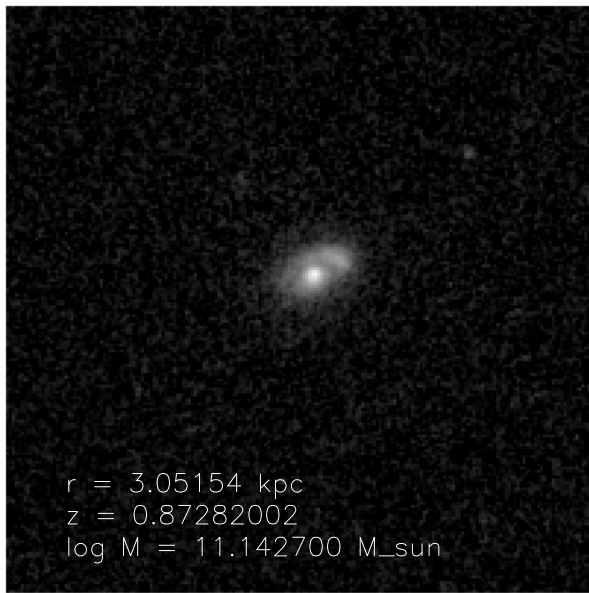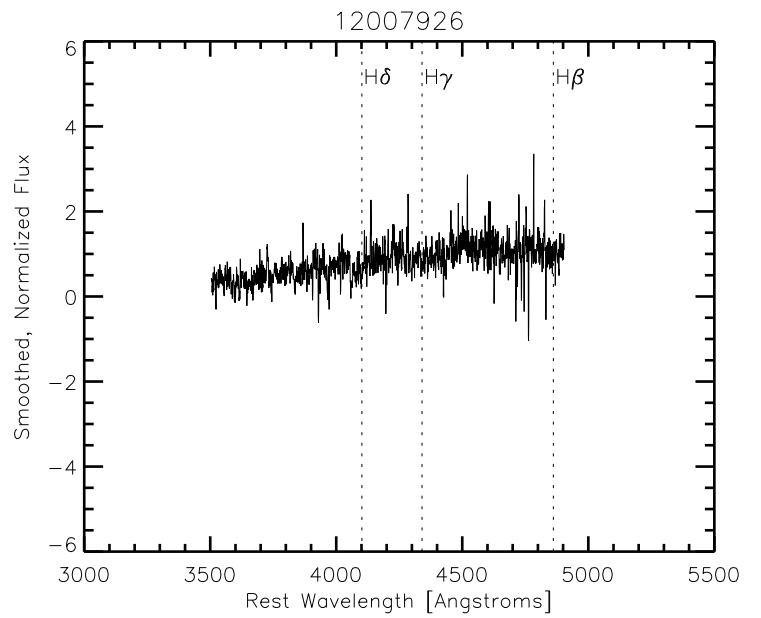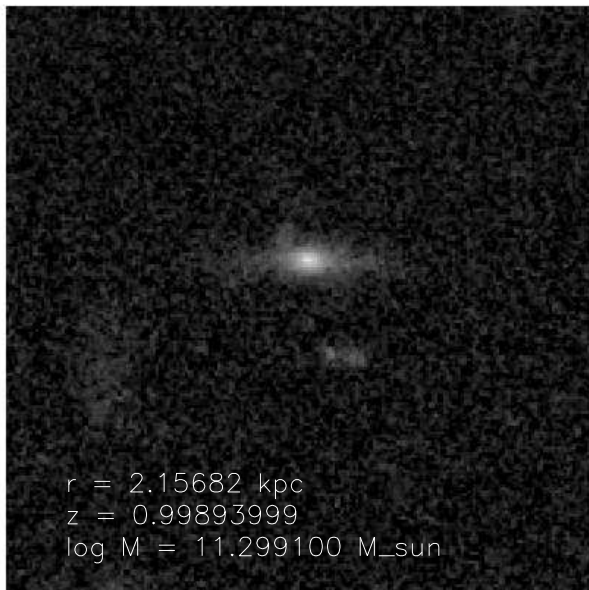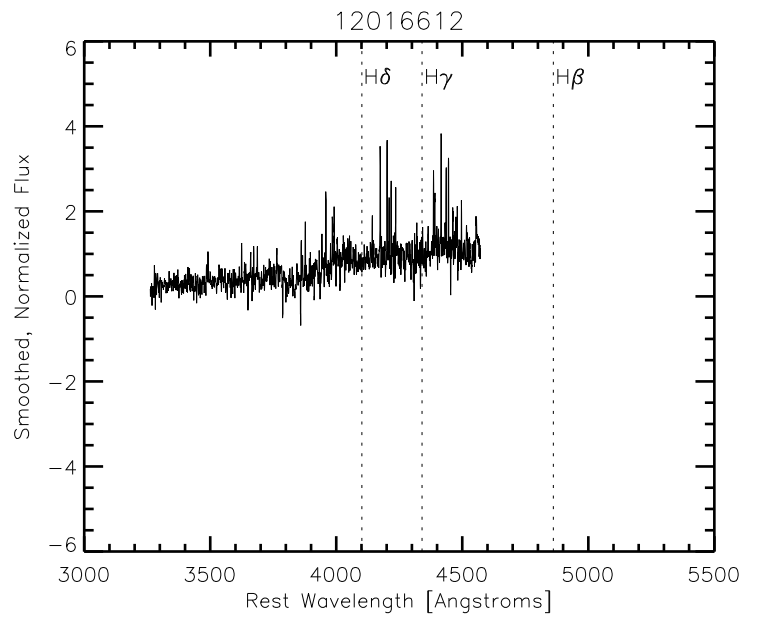

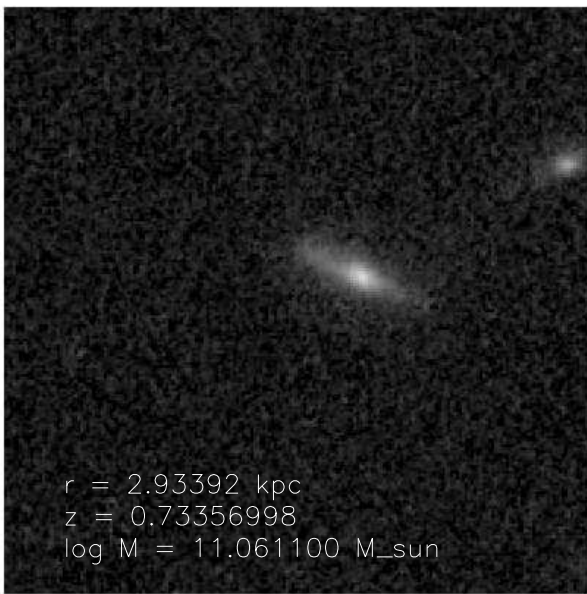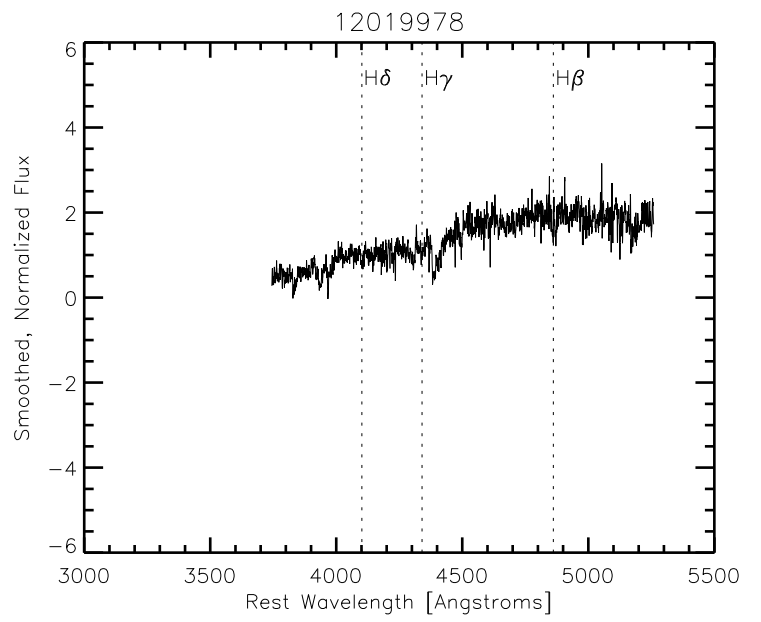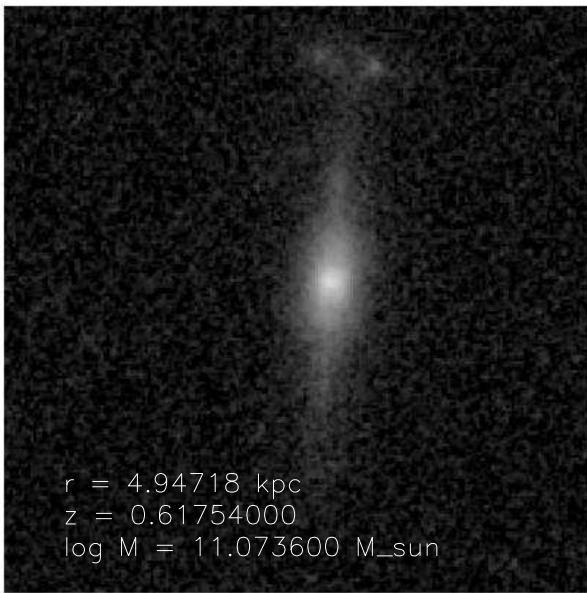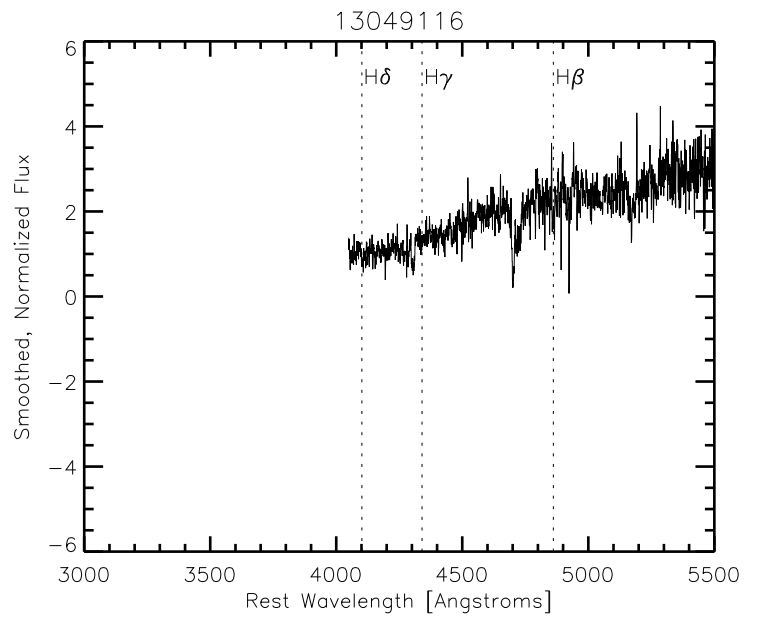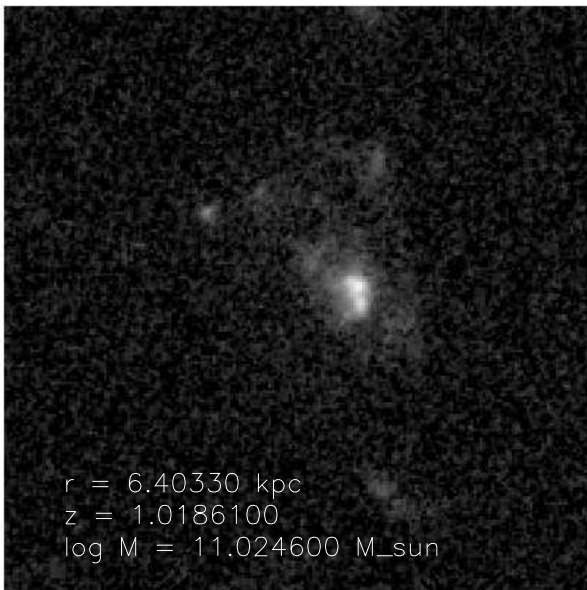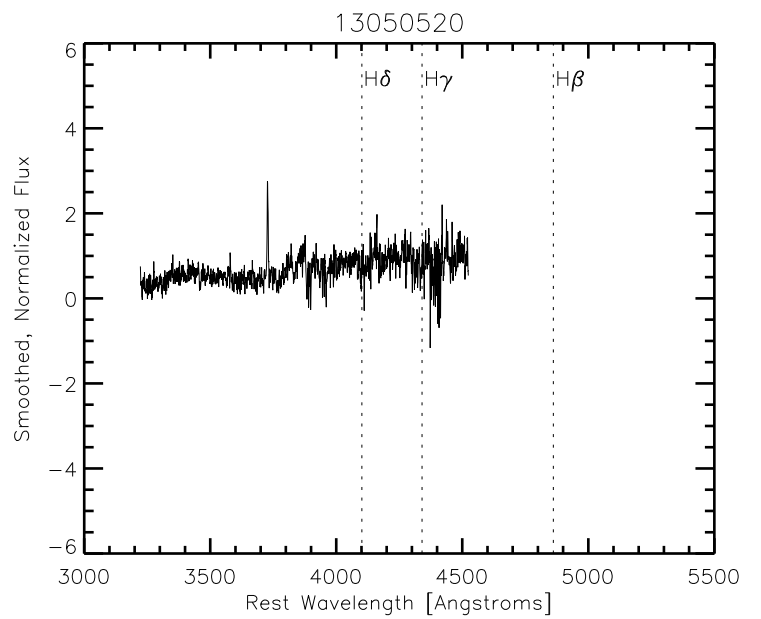

Supplement: Supplementary file 1 [file appendix_b1.pdf]
